# Supplementary material for: Visualizing Movement Control Optimization Landscapes
Source: arXiv:1909.07869 source file (2020-08-22)
Supplement: Supplementary file 1 [file appendix.tex]

%!TEX root = main.tex

%=======================================================================
\section{Properties and limitations of random 2D slice visualizations}\label{sec:theory}
In the preceding sections, we have provided many examples of random 2D slice visualizations of high-dimensional objective functions. We have also demonstrated that such visualizations can predict the difficulty of optimization. However, as information is obviously lost in only evaluating the objective along a 2D slice, one may pose the following research question: 
%Figure \ref{fig:randomslices} illustrates how random 2D slice visualizations of the inverted pendulum trajectory optimization objective of Equation \ref{eq:trajcost} are quite consistent and display relevant characteristics of the objective. All the visualizations show some non-convexity, multimodality and ill-conditioning of the global optimum in the middle. However, as information is obviously lost in only evaluating the objective along a 2D slice, one may pose the following research question: 

\textit{How reliable are random 2D visualizations as a diagnostic tool for indicating problems like ill-conditioning and multimodality?} 

In this section, we investigate this question using test functions with known properties and closed-form expressions. This yields the following main results:

\begin{itemize}
\item There is no guarantee that ill-conditioning and multimodality will show up in a random visualization slice.
\item On the other hand, if ill-conditioning or multimodality do show up, they are real. This mitigates the limitation above and makes random 2D slice visualizations a useful tool for analyzing optimization problems.
\end{itemize}

In other words, \textit{as a diagnostic tool for identifying problems, random 2D visualizations have low sensitivity compensated by high specificity}.

%Considering the above, it may be that random 2D slices provide a highly limited view of an optimization problem. On the other hand, Figure \ref{fig:randomslices} illustrates how random 2D slice visualizations of the inverted pendulum trajectory optimization objective of Equation \ref{eq:trajcost} are quite consistent and informative. All the visualizations display the multimodality and elongation of the global optimum in the middle. To better understand the reliability of such visualizations, we will now further investigate the limits of visualizing ill-conditioning and multimodality.

\subsection{Visualizing ill-conditioned optima}
As elaborated below, the number of high and low eigenvalues of the Hessian greatly affects visualization in addition to the condition number, i.e., ratio of highest and lowest eigenvalues.

Consider the following cost function with \textit{intrinsic dimensionality $k$}:  

\begin{eqnarray}
f(\mathbf{x})&=&\sum_{i=1}^{k} x_i^2 + \sum_{i=k+1}^{d} \epsilon x_i^2\\
&=& ||\mathbf{x}_{:k}||^2 + \epsilon ||\mathbf{x}_{k:}||^2 \label{eq:kd}
\end{eqnarray}

where $\epsilon$ is a small constant, i.e., $f(\mathbf{x})$ mostly depends only on the first $k$ optimized variables. $\mathbf{x}_{:k}$ denotes the projection of $\mathbf{x}$ into the subspace of the first $k$ dimensions. $\mathbf{x}_{k:}$ denotes the projection into the remaining dimensions. The Hessian of $f(\mathbf{x})$ is diagonal, containing the curvatures along the unit vectors as the diagonal elements. Curvature along the first $k$ unit vectors equals $2$ and curvature along the rest of the dimensions is $2\epsilon$. Thus, if $k \neq 0$ and $k \neq d$, the condition number $\kappa = 1/\epsilon$. 

Geometrically, the isosurfaces of $f(\mathbf{x})$ are $n$-spheres elongated by a factor of $1/\sqrt{\epsilon}$ along the last $d-k$ dimensions. The visualized 2D isocontours correspond to the intersections of the isosurfaces with the visualization plane. This is illustrated in Figure \ref{fig:isosurfaces} and on the supplemental video for $d=3$.

\begin{figure}[h]
\centering
\includegraphics[width=3.4in]{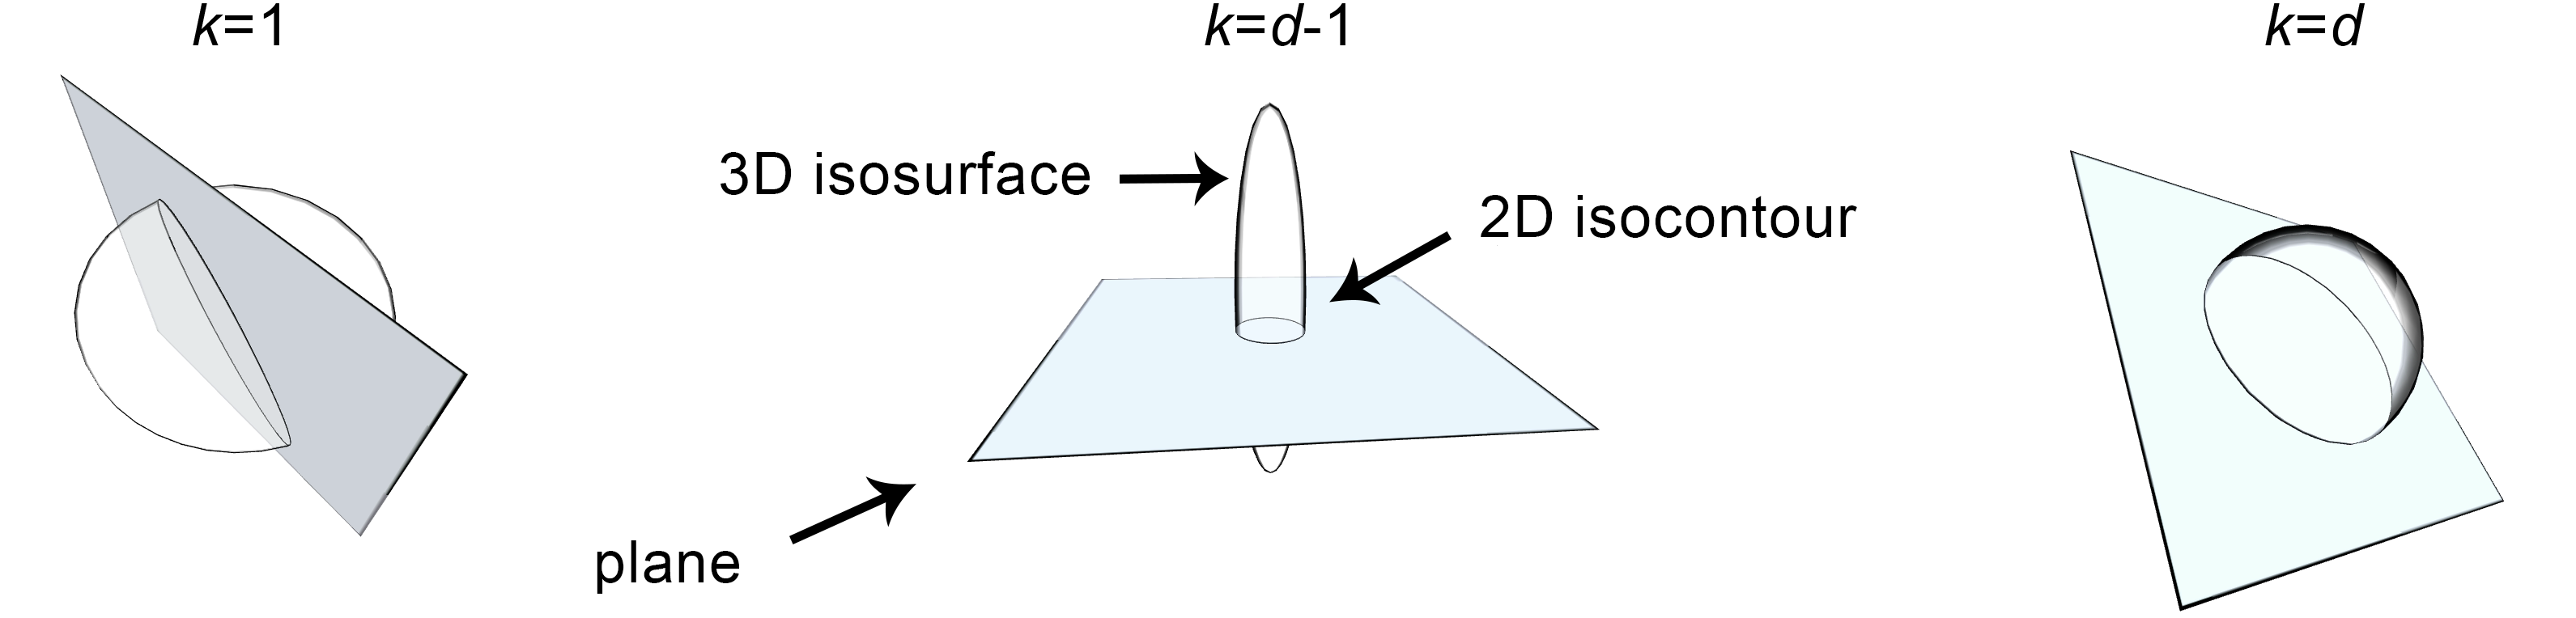}
\caption{The isosurfaces, random visualization planes, and 2D visualization isocontours for Equation \ref{eq:kd} in the case of $d=3$.}\label{fig:isosurfaces}
\end{figure}

Investigating Figure \ref{fig:isosurfaces} reveals a basic property of the 2D visualizations:

\textbf{Proposition 1} \textit{With an objective function of the form of Equation \ref{eq:kd}, the elongation of the 2D isocontours is less than or equal to the true elongation of the isosurfaces. In other words, $\kappa_{2D} \le \kappa$}

\textit{Proof.} The proof follows from the isocontours corresponding to planar intersections of the isosurfaces. First, as illustrated in the middle of Figure \ref{fig:isosurfaces}, it is possible to rotate the visualization plane such that the isocontours display less elongation. Second, the isocontours cannot display more than the real elongation; the visualized elongation is at maximum when one plane basis vector aligns with a direction of high elongation (vertical axis in the middle of Figure \ref{fig:isosurfaces}), and the other basis vector aligns with a direction of low elongation, in which case the isocontours display the correct $\kappa = 1/\epsilon$ $\qed$

%illustrates how even if a random 2D visualization shows a well-conditioned objective -- e.g., in the middle of the figure -- the reality may be worse. On the other hand, it is possible to rotate the visualization plane such that it aligns with both the maximal and minimal axes of elongation and thus displays the true ill-conditioning. These observations can be stated as a proposition
%The visualized elongation is at maximum when the plane aligns with the dimensions where the isosurface is the widest and narrowest,

%The case $k=d$ in Figure \ref{fig:isosurfaces} is simple and can be formally stated as:

%\textit{Proof.} The isosurfaces of a spherical function are $n$-spheres. The isocontours of the visualization are intersections of the visualization plane and the $n$-spheres, i.e., circles. $\qed$

%If $k=d-1$, cost is low only near the last unit vector. If $k=1$, cost is low inside the hyperplane comprising the last $d-1$ dimensions, and cost grows rapidly only when moving along the first unit vector, i.e., the normal of the hyperplane.

A crucial observation from Figure \ref{fig:isosurfaces} is that the number of possible visual plane rotations that display ill-conditioning depends on $k$. When $k=1$, the isocontours are mostly highly elongated, except when the visualization plane is aligns with the lens-shaped isosurface. In contrast, with $k=d-1$, the 2D isocontours are mostly not showing the true elongation of the isosurface, except when the visualization plane aligns with the axis of elongation. 

For a more formal analysis of how the visualization depends on $k$, let us consider the extreme case of $\epsilon = 0$, i.e.,  

\begin{equation}
f(\mathbf{x}) = f(\mathbf{x}_{:k}) = ||\mathbf{x}_{:k}||^2.  \label{eq:kdapprox}
\end{equation}

Figure \ref{fig:kd} shows the contour plots of random 2D slices with different $k$ and $d$, motivating the following proposition:

\textbf{Proposition 2} \textit{As $k$ moves from 1 to $d$, the condition number of a random 2D slice visualization of $f(\mathbf{x})$ moves from $\infty$ to 1, with random variation between the extremes.}

\textit{Proof.} Let $\mathbf{u}, \mathbf{v} \in \mathbb{R}^d$  denote the slice basis vectors, with orthogonality $\mathbf{u}^T\mathbf{v}=0$. On the visualization plane, $\mathbf{x}=p_1 \mathbf{u} + p_2 \mathbf{v} = [\mathbf{u} \mathbf{v}]\mathbf{p}$, where $\mathbf{p}$ denotes the 2D position on the plane. Similarly, $\mathbf{x}_{:k}=[\mathbf{u}_{:k} \mathbf{v}_{:k}]\mathbf{p}$, 

\begin{eqnarray}
f(\mathbf{x}_{:k}) &=& ||[\mathbf{u}_{:k} \mathbf{v}_{:k}]\mathbf{p}||^2\\
&=& \mathbf{p}^T \begin{bmatrix}
\mathbf{u}^T_{:k}\mathbf{u}_{:k} & \mathbf{u}^T_{:k}\mathbf{v}_{:k} \\
\mathbf{v}^T_{:k}\mathbf{u}_{:k} & \mathbf{v}^T_{:k}\mathbf{v}_{:k}
\end{bmatrix} \mathbf{p} \\
&=& \mathbf{p}^T \mathbf{A} \mathbf{p}
\end{eqnarray}

The Hessian w.r.t. $\mathbf{p}$ of the quadratic form is

\begin{eqnarray}
H(f(\mathbf{x}_{:k}))=\mathbf{A}+\mathbf{A}^T=2\mathbf{A}
\end{eqnarray}

because $\mathbf{A}$ is symmetric. The condition number $\kappa(H(f(\mathbf{x}_{:k}))=\kappa(\mathbf{A})$, as the condition number is invariant to scaling the Hessian by a constant. Thus, it is sufficient to analyze how $\mathbf{A}$ changes when $k$ moves from 1 to $d$. 

With $k$=1, $\mathbf{u}_{:k}=u_1, \mathbf{v}_{:k}=v_1$ are scalars, and the determinant becomes zero:

\begin{eqnarray}
\det(\mathbf{A})&=& \mathbf{u}^T_{:k}\mathbf{u}_{:k}\mathbf{v}^T_{:k}\mathbf{v}_{:k} - \mathbf{u}^T_{:k}\mathbf{v}_{:k}\mathbf{v}^T_{:k}\mathbf{u}_{:k} \\
&=&u_1 u_1 v_1 v_1 - u_1 v_1 v_1 u_1 = 0.
\end{eqnarray}

This indicates at least one zero eigenvalue and thus $\kappa(\mathbf{A})=\max(eig(\mathbf{A}))/\min(eig(\mathbf{A}))=\infty$.

When $k$ grows from 1 to $d$, $\mathbf{u}_{:k}, \mathbf{v}_{:k}$ gradually become closer to $\mathbf{u}, \mathbf{v}$, i.e., unit-length and orthogonal. Thus, the off-diagonal elements become zero and $\mathbf{A}$ becomes the identity matrix, with $\kappa(\mathbf{A})=1$. $\qed$ 

Although the quadratic $f(\mathbf{x})$ was chosen to be separable for easier mathematical analysis, the propositions above generalize to the arbitrarily rotated case.

Considering Figure \ref{fig:kd} and the propositions above, one may articulate the following conclusions:

\begin{itemize}
\item A random 2D slice visualization may not display ill-conditioning if the optimization problem has high intrinsic dimensionality $k$. 
\item On the other hand, the visualizations will not show non-existent problems; spherical functions will appear spherical and the intersection of the plane and an isosurface cannot show more elongation than the isosurface has. Thus, the visualization can still be useful in highlighting problems, which is also supported by the the empirical data in this paper. Furthermore, while higher intrinsic dimensionality makes ill-conditioning harder to visualize, it also decreases the severity of the problem, as one can get closer to the true optimum even if the optimizer only focuses on the intrinsic dimensions.  
\end{itemize}

%However, the visualizations are is still a viable tool due to the high specificity; any ill-conditioning that is captured is real and not imaginary. In case of $d=k$, the isosurfaces are spheres and the 2D isocontours are circles, correctly displaying a well-conditioned objective.

\begin{figure}[h!]
\centering
\includegraphics[width=3.4in]{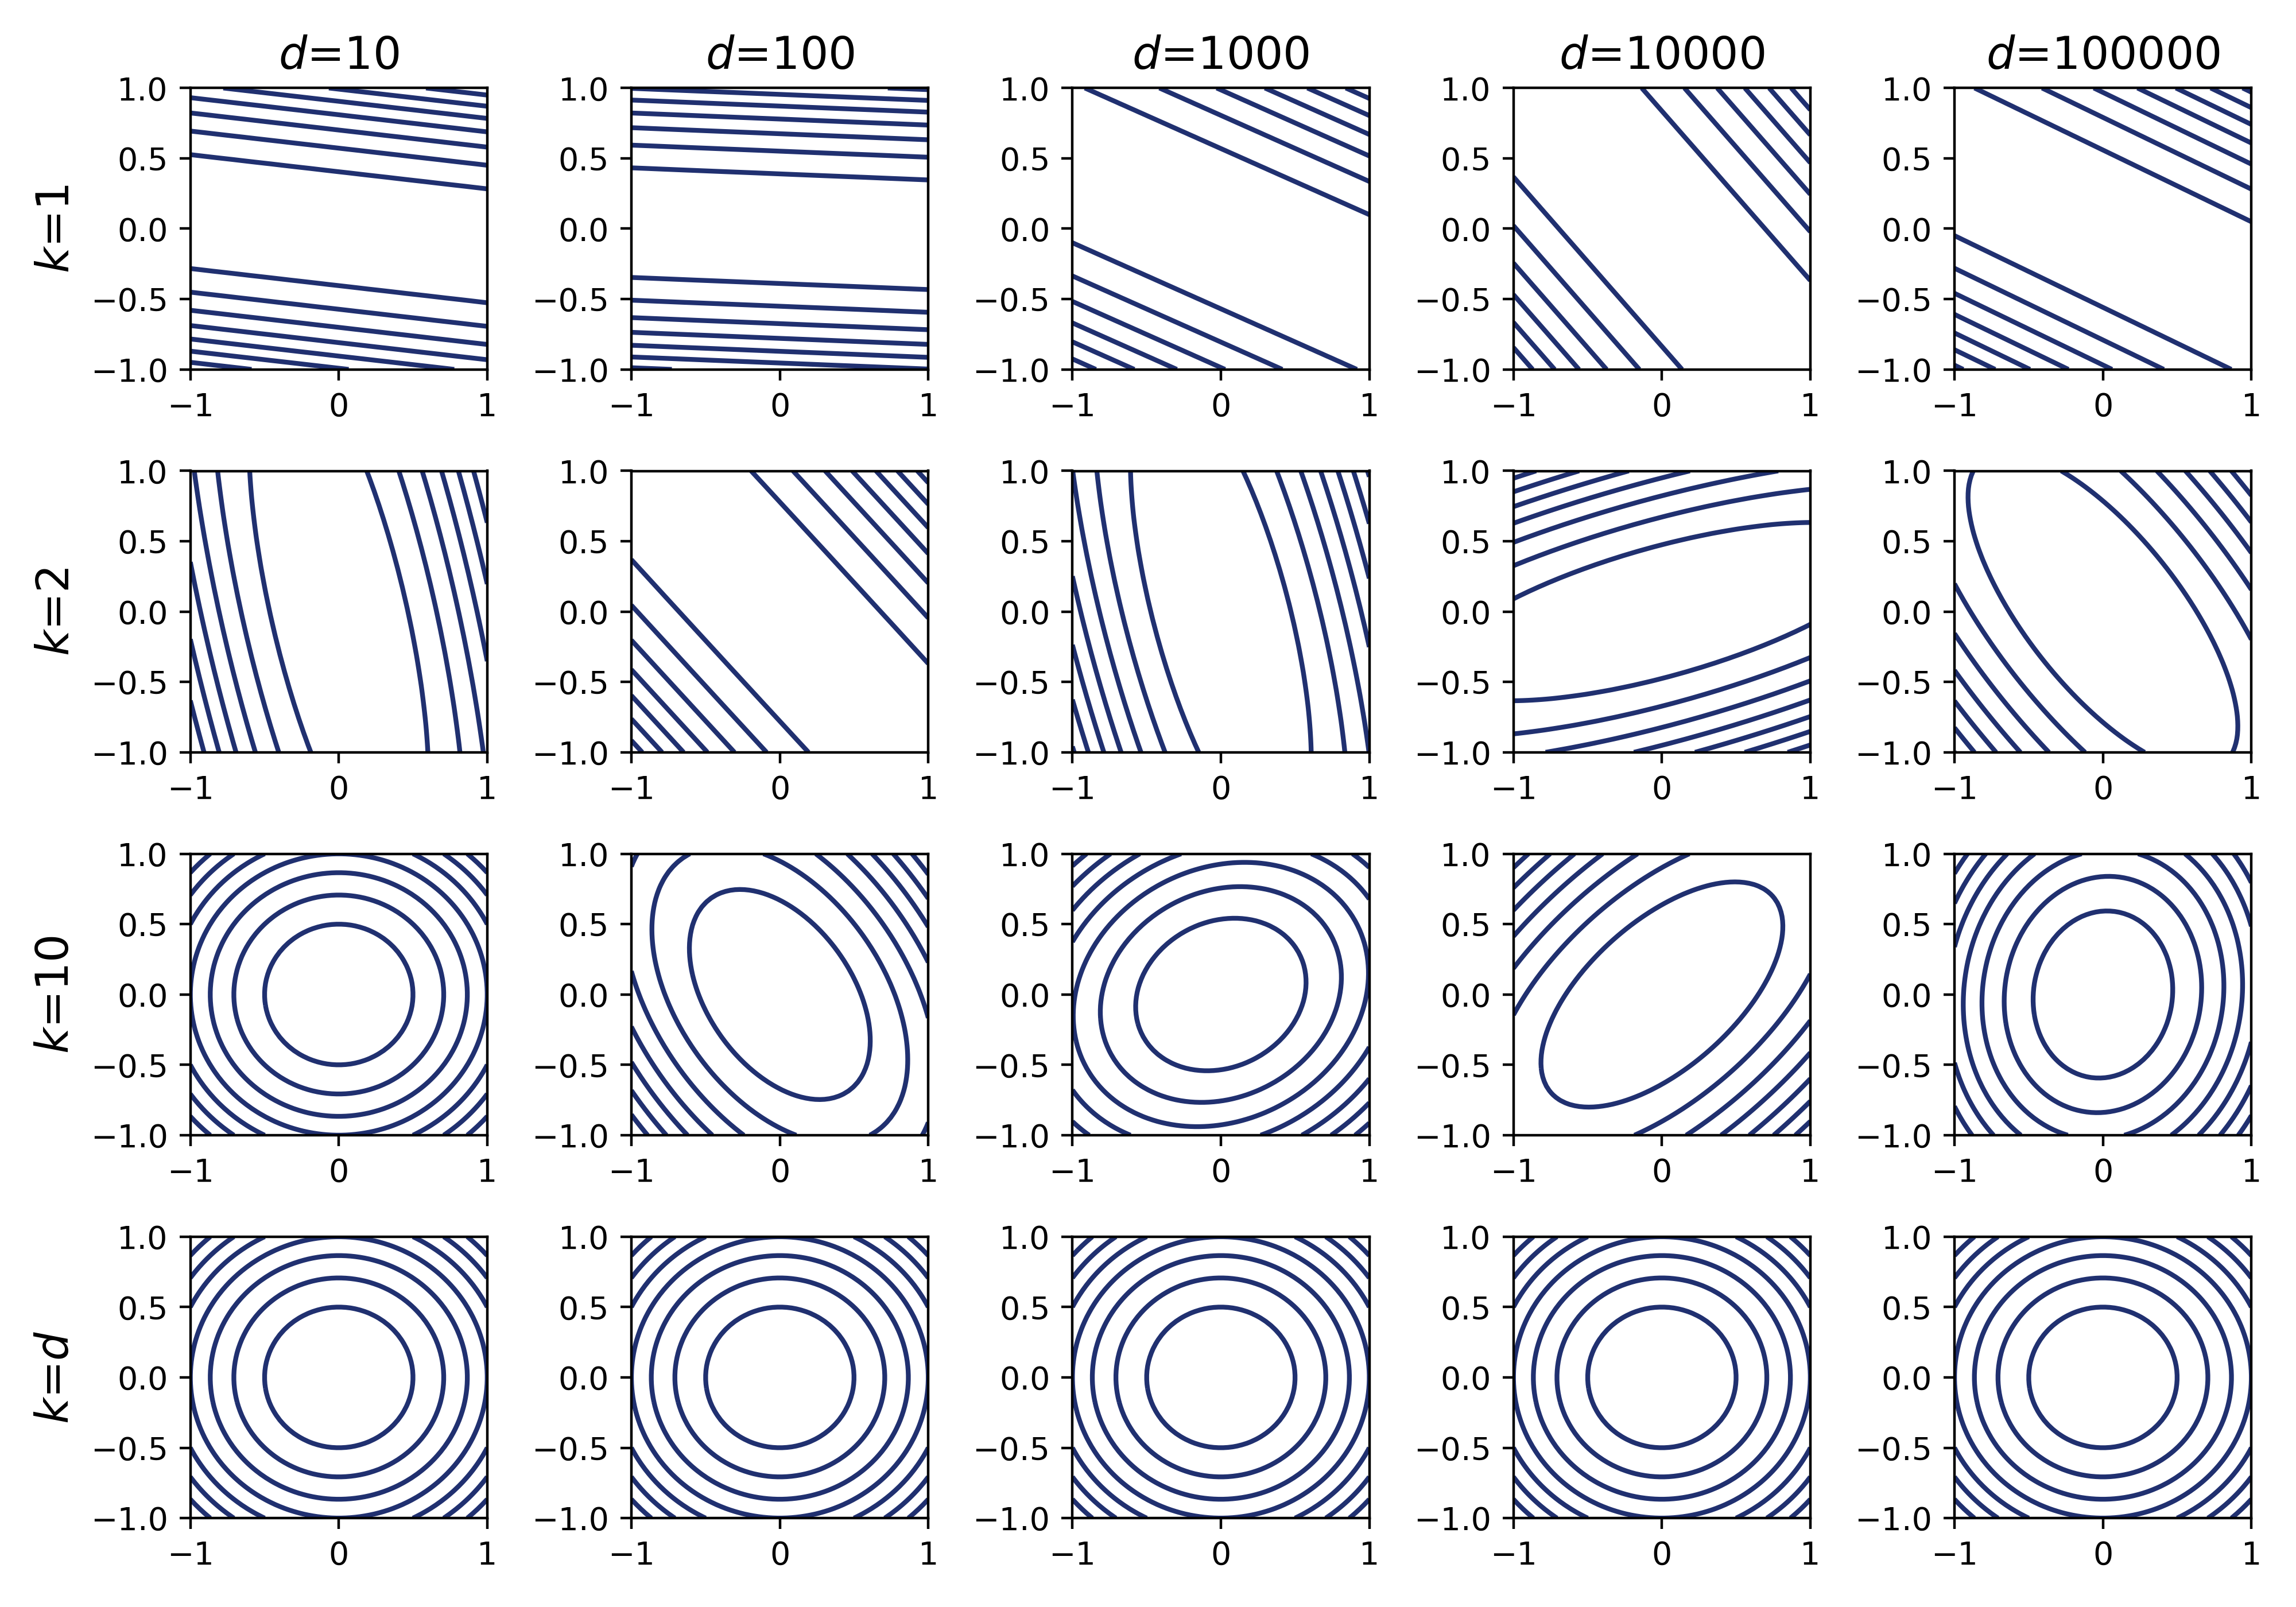}
\caption{Contour plots of random slices of $f(\mathbf{x})$ in Equation \ref{eq:kd} with different $k$ and $d$. As $k$ grows towards $d$, ill-conditioning becomes less apparent in the visualization. }\label{fig:kd}
\end{figure}

\paragraph{Relation to random projection theory.} Our visualized 2D isocontours are determined by intersecting a randomly selected plane (a 2D subspace) with high-dimensional isosurfaces. Interestingly, random projection theory deals with a related operation of projecting high-dimensional data on random subspaces. A central result, in line with our findings, is that if data clusters are highly eccentric (non-spherical), projecting the data to a random low-dimensional subspace will make them appear more spherical \cite{dasgupta1999learning, dasgupta2013experiments}. 

\subsection{Visualizing multimodality}
Figure \ref{fig:nonconvex} shows contour plots of random visualization slices with different dimensionality $d$, using two multimodal test functions. Rastrigin's function is a standard multimodal optimization test function with the global minimum at the origin and infinitely many local minima:

\begin{equation}
f_{Rastrigin}(\mathbf{x})=10d+\sum_{i=1}^d [x_i^2-10\cos(2\pi x_i)]
\end{equation}

Additionally, we use the following bimodal function:

\begin{equation}
f_{Bimodal}(\mathbf{x})=e^{-\frac{1}{2}||\mathbf{x}-\mathbf{1}||^2} + 0.8e^{-\frac{1}{2}||\mathbf{x}+\mathbf{1}||^2},
\end{equation}

where the boldface $\mathbf{1}$ denotes a vector of ones. We visualize this function both around the origin and around the dominant mode at $\mathbf{1}$. 

From Figure \ref{fig:nonconvex}, one may draw the following conclusions:

\begin{itemize}
\item Multimodality may become less apparent with increasing dimensionality. Additionally, if there are only a few modes, it may easily happen that modes collapse together in the visualization.
\item With the bimodal function, visualization appears more unimodal when computed around the optimum at $\mathbf{1}$. This can be explained by the norm of the other mode having less influence near the optimum, as the Euclidian distance between the optima grows with dimensionality.
\item With functions like Rastrigin, landscape features may scale differently. Rastrigin's central mode becomes larger and more dominant with large $d$. In Figure \ref{fig:nonconvex}, we demonstrate how this can be compensated by omitting the unit-length normalization of the slice basis vectors, and instead normalizing them to the mean of their original lengths. We also demonstrate that high-pass filtering the 2D-array of function values before plotting can bring back detail that would otherwise become invisible with large $d$.
\end{itemize}

\begin{figure}[h]
\centering
\includegraphics[width=3.4in]{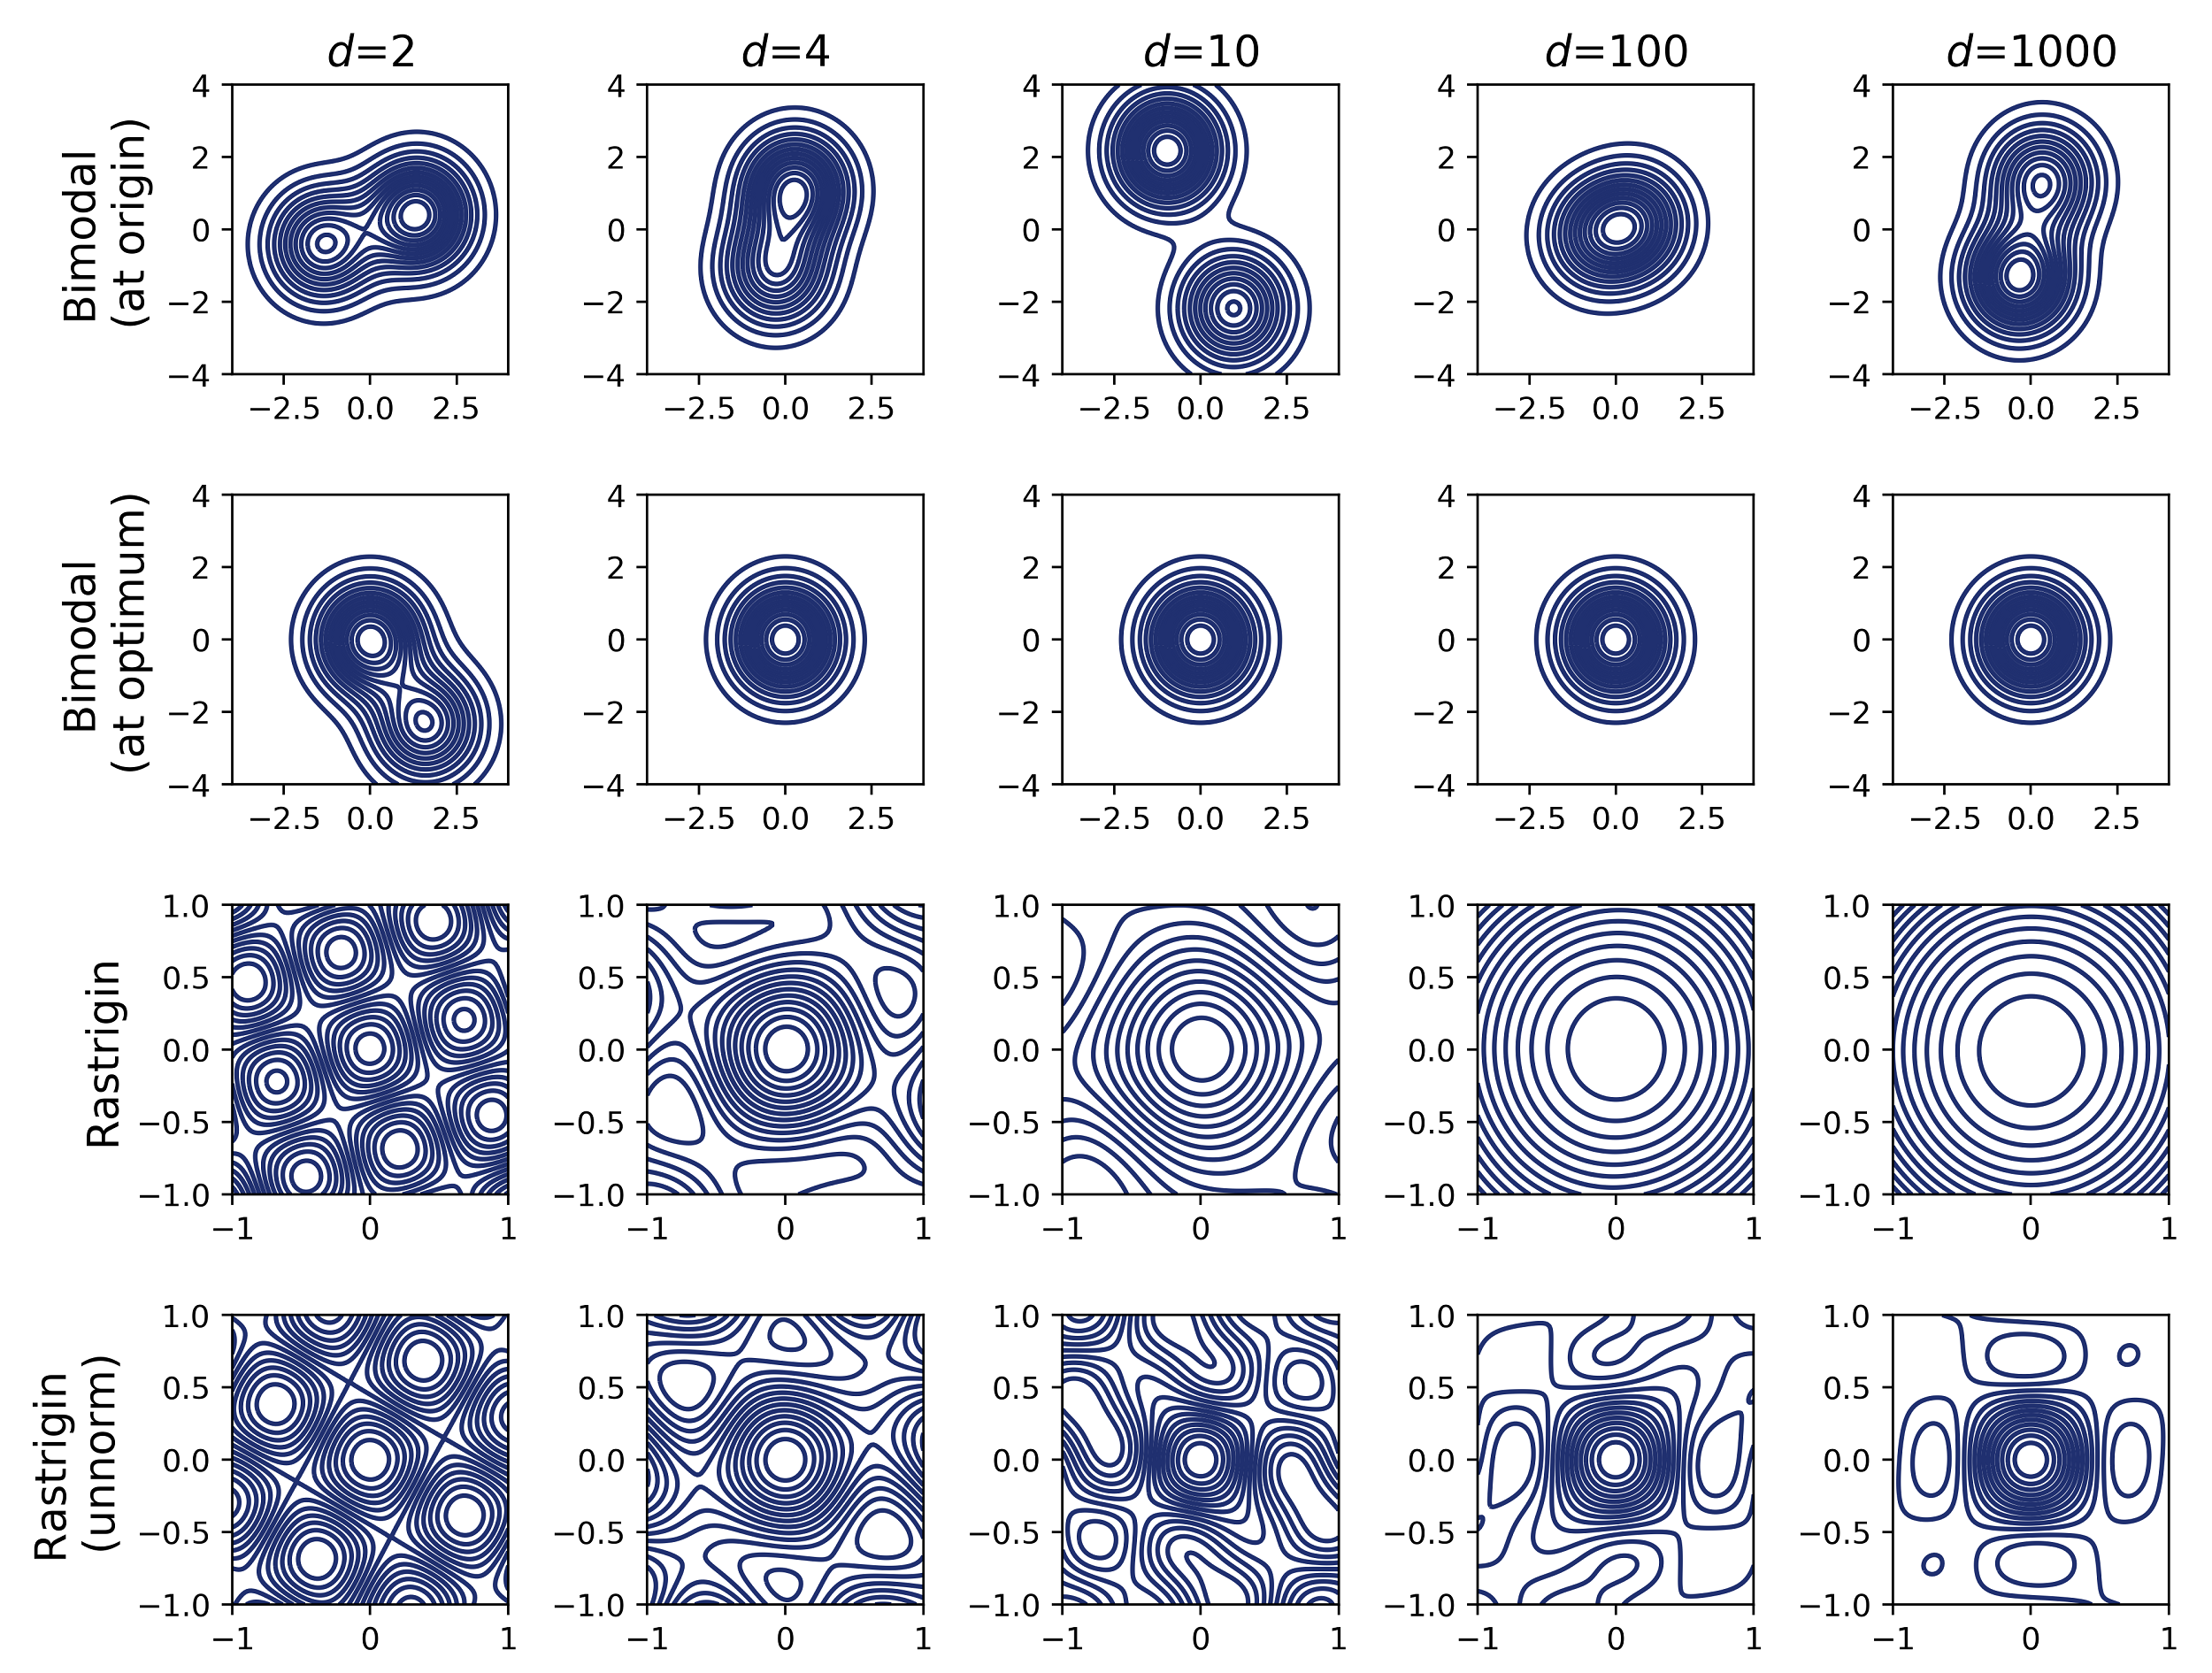}
\caption{Contour plots of random slices of multimodal test functions with different $d$. Large $d$ can make multimodality less apparent, although it can be compensated by using unnormalized visualization basis vectors or high-pass filtering. }\label{fig:nonconvex}
\end{figure}

In summary, considering both Figure \ref{fig:kd} and Figure \ref{fig:nonconvex}, random 2D slice visualizations can help in characterizing optimization landscapes and identifying problems. However, for some function types like an elongated quadratic with high intrinsic dimensionality, the visualizations may be overly optimistic.
